# Supplementary material for: A nanofocused plasmon-driven sub-10 femtosecond electron point source
Source: arXiv:1512.07037 ancillary file (2016-03-03)
Supplement: Supplementary file 1 [file Mueller_arxiv1512.07037_supportingInfo.pdf]

# A nanofocused plasmon-driven sub-10 femtosecond electron point source

# Supporting Information

Melanie Müller[1], Vasily Kravtsov[2], Alexander Paarmann[1], Markus B. Raschke[2] and Ralph Ernstorfer[1]

*[1] Fritz-Haber-Institut der Max-Planck-Gesellschaft, Faradayweg 4-6, 14195 Berlin, Germany*

*[2] Department of Physics, Department of Chemistry, and JILA, University of Colorado, Boulder, Colorado 80309, USA*

Corresponding Author: ernstorfer@fhi-berlin.mpg.de

4 pages, 2 figures

We provide additional discussion of the electron lens principle and its application for identification of the electron emission sites. We perform fully 3D numerical simulations to calculate the electrostatic properties as well as the particle trajectories using a finite element method (COMSOL Multiphysics 5.1). We compare our simulations to data from a tip which in addition to plasmon-driven electron emission also shows direct photoemission from the grating structure, verifying nanofocused plasmonic electron emission.

The simulations are based on the typical geometry of the tip-lens assembly[1], see Figure S1.a). The tip has a radius of 30 nm, a half opening angle of 10° and protrudes the lens by 250 µm, which has an outer diameter of 100 µm. The tip is biased at -500 V and the grounded anode is positioned at a distance $d$ = 775 µm below the tip. Figure S1.b) plots the electric potential $U$ in the $y$-$z$-plane between the lens and a distance $z$ = 200 µm below the apex for a lens voltage $U_L$ = -840 V. To illustrate the effect of the lens voltage on the electric field distribution, Figures S1.c) and S2.d) plot the electric potential in close proximity of the tip apex for two lens voltages $U_L$ = -840 V and $U_L$ = -860 V, respectively. At low lens voltage the potential distribution approaches that of a lens-less tip[2] (not shown here). At (negatively) increasing lens voltage the field lines close to the apex are flattened and eventually bend in the opposite direction, accompanied by a reduction and eventual sign reversal of the electric field. Likewise, the electric field at positions higher along the tip shaft is reduced and reverses sign at a characteristic lens voltage. The dependence of the normalized electric field $E_n$ on $U_L$ is plotted in Figure S1.d) for three shaft positions and at the apex.

Electron beam profiles are then calculated depending on the lens voltage for electrons emitted from the apex and for different emission sites along the tip shaft. To account for the energy spread upon photoemission, the initial electron energy is modeled by a Gaussian distribution with a mean energy of $E_0$ = 0.1 eV and a width of $\sigma_E$ = 0.5 eV [3]. The values are chosen according to typical values for multiphoton emission found in the literature[3], neglecting plasmonic acceleration justified by the low electric field strength below 1 GV/m [4]. The spatial distribution of emission sites are modeled by 2D gaussian distributions of the emission probability, with standard deviations of $\sigma_x = \sigma_y$ = 10 nm at the apex, and $\sigma_x$ = 600 nm and $\sigma_z$ = 10 nm at the shaft positions, respectively.. The electron's final position is then analyzed at the anode in the $x$-$y$-plane.

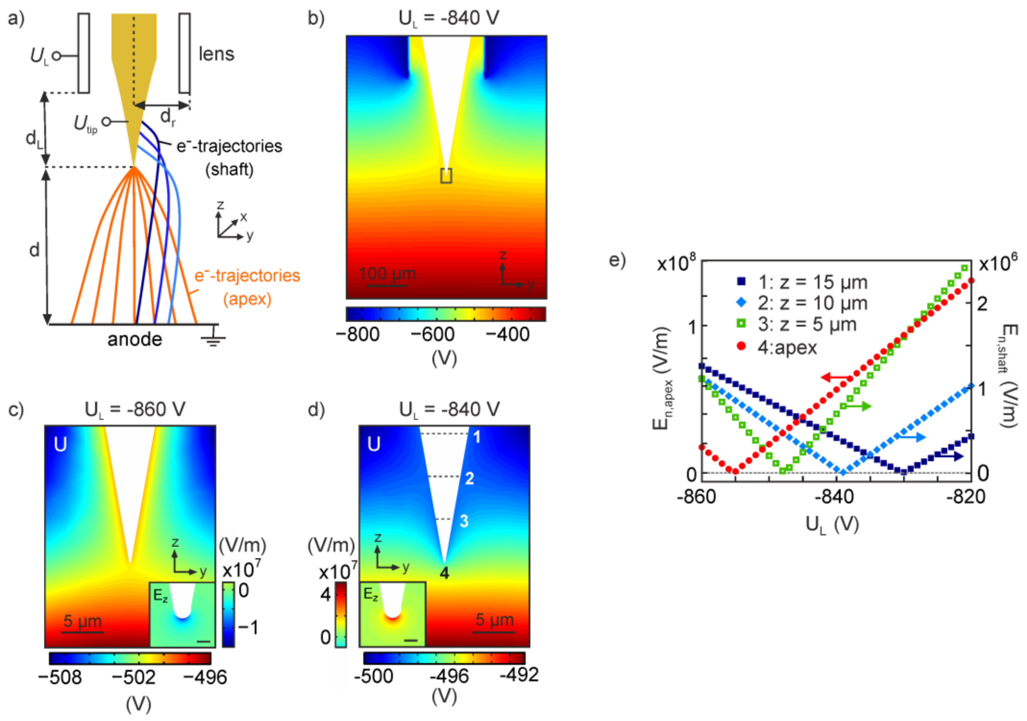

**Figure S1.** Electrostatic simulation of the tip-lens assembly. (a) Tip-lens geometry with grounded anode at a distance *d* below the tip, which protrudes the lens by $d_L$ having an outer diameter $d_r$. Electron trajectories originating from the tip apex and different shaft positions are sketched for illustration. (b) Electrostatic potential $U$ at $U_{tip}$ = -500 V and $U_L$ = -840 V between lens and 200 µm below the tip apex plotted in the *y*-*z*-plane. (c) and (d) show the calculated electric potential $U$ for two lens voltages $U_L$ = -840 V and $U_L$ = -860 V, respectively, in close proximity of the apex (corresponding to the drawn box in (b)). Insets: z-component $E_z$ of the electric field at the apex (scale bars: 50 nm). (d) Normalized electric field $E_n$ at the apex (red circles, left y-axis) and at three positions along the shaft (right y-axes) corresponding to numbers 1-4 in (d).

To verify plasmon-induced electron emission from the apex, we compare the focused spot profiles of apex electrons with those emitted from the tip shaft, which we observe for some of our tips. Figure S2.a) shows the emission profiles of such an imperfect tip for apex (top) and grating illumination (bottom), at $U_{tip}$ = -500 V and for four different lens voltages. When illuminating the grating, we observe the same general spot profile as in the case of direct apex illumination (nearly homogeneous spot), but superimposed by a distinct arc-shaped profile. The arc-shaped contribution is highly asymmetric with respect to the tip axis and focuses within a narrower range of lens voltages. We identify these electrons to originate from the shaft by comparison with simulated electron distributions.

In Figure S2.b) we plot the mean radial distance $\langle r_{det} \rangle$ of the calculated electron position in the detector plane. For shaft electrons (squares) we observe a minimum of $\langle r_{det} \rangle$ in the anode plane at a characteristic focusing voltage $U_{L,foc}$ which depends linearly on the z-coordinate $z_{rel}$ of the

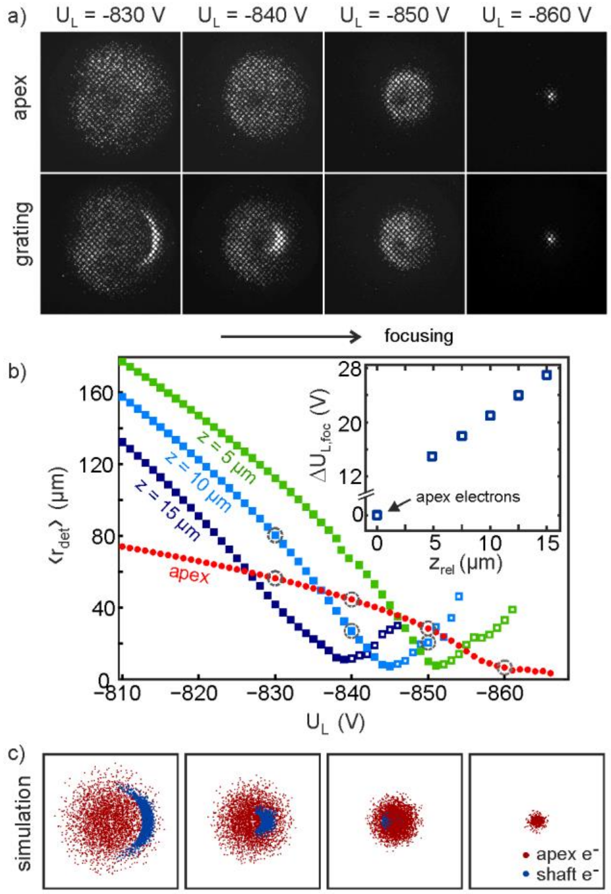


**1Figure S2.** Identification of the electron emission sites, exemplified for an imperfect nanotip. (a) Spot profile analysis of electrons emitted from the apex and from the grating. Emission profiles for apex (top) and grating illumination (bottom) for four different lens voltages ($U_{tip}$ = -500 V) of a tip showing plasmon-induced emission from the apex (homogeneous spot) as well as direct photoemission at the grating coupler (arc-shaped feature) in the case of grating illumination. (b) Mean radial distance $\langle \boldsymbol{r}_{\mathbf{det}} \rangle$ of simulated spot profiles for apex emission (red circles) and three positions along the shaft (squares) analyzed in the detector plane. The inset shows the linear dependence of the focusing voltage (relative to the focusing voltage at the apex), $\Delta U_{L,foc}$ , on the z-coordinate of the emission site. At voltages more negative than $\Delta U_{L,foc}$ electrons from the shaft are defocused again (open squares). (c) Superimposed simulated spot profiles of electrons originating from the apex (red) and from $z_{shaft}$ = 10 µm at the tip shaft (blue) for the same voltages as in (a), and corresponding to the dotted circles in (c).

emission site relative to the apex (as plotted in the inset). In particular, a beam crossover is observed for electrons originating from the shaft, which is not the case for electrons emitted from the apex (red circles). In all cases, electron emission is suppressed completely at a certain lens voltage due to the sign reversal of the electric field. The superimposed calculated spot profiles of apex (red) and shaft electrons (blue, from $z_{shaft}$ = 10 µm) are plotted in Figure S2.c). We can therefore clearly assign the distinct asymmetric arc-shaped emission to direct photoemission from the grating, and in turn identify the homogeneous emission spot in Figure 2 as plasmon-triggered electron emission purely from the apex.

In general, the focusing behavior $\langle r_{\mathrm{det}} \rangle (U_L)$ and in particular the width of the arc-shaped profile depends on the initial energy of the photoelectron, which in principle can be modified by the plasmonic near field at high enough field strength[4]. However, independent of the initial energy distribution, electron emission from the tip shaft always results in highly asymmetric profiles and much stepper slopes of $\langle r_{\mathrm{det}} \rangle (U_L)$. This allows for identification of emission sites without exact knowledge of the initial electron distribution.

## References


1. Müller, M.; Paarmann, A.; Ernstorfer, R. Femtosecond electrons probing currents and atomic structure in nanomaterials. *Nature Comm.* **2014**, 5, 5292.

2. Paarmann, A.; Gulde, M.; M□uller, M.; Sch□afer, S.; Schweda, S.; Maiti, M.; Xu, C.; Hohage, T.; Schenk, F.; Ropers, C.; Ernstorfer, R. Coherent femtosecond low-energy single-electron pulses for time-resolved diffraction and imaging: A numerical study. *J. Appl. Phys.* **2012**, 112, 113109.

3. Yanagisawa, H.; Hengsberger, M.; Leuenberger, D.; Klöckner, M.; Hafner, C.; Greber, T.; Osterwalder, J. Energy Distribution Curves of Ultrafast Laser-Induced Field Emission and Their Implications for Electron Dynamics. *Phys. Rev. Lett.* **2011**, 107, 087601.

4. Rácz, P,; Dombi, P. Nonponderomotive electron acceleration in ultrashort surface-plasmon fields, *Phys. Rev. A* **2011**, 84, 063844.
